# Supplementary material for: Learning Descriptive Image Captioning via Semipermeable Maximum Likelihood Estimation
Source: arXiv:2306.13460 source file (2023-10-28)
Supplement: Supplementary file 1 [file rebuttal_supplementary.tex]

\begin{center}
\Large{\textbf{Response Supplementary for Learning Descriptive Image Captioning via Semipermeable Maximum Likelihood Estimation}}
\end{center}

\appendix

\section{Quantitative Results of Human Evaluation}

\begin{figure}[h]
	\begin{center}
		\includegraphics[width=1\linewidth]{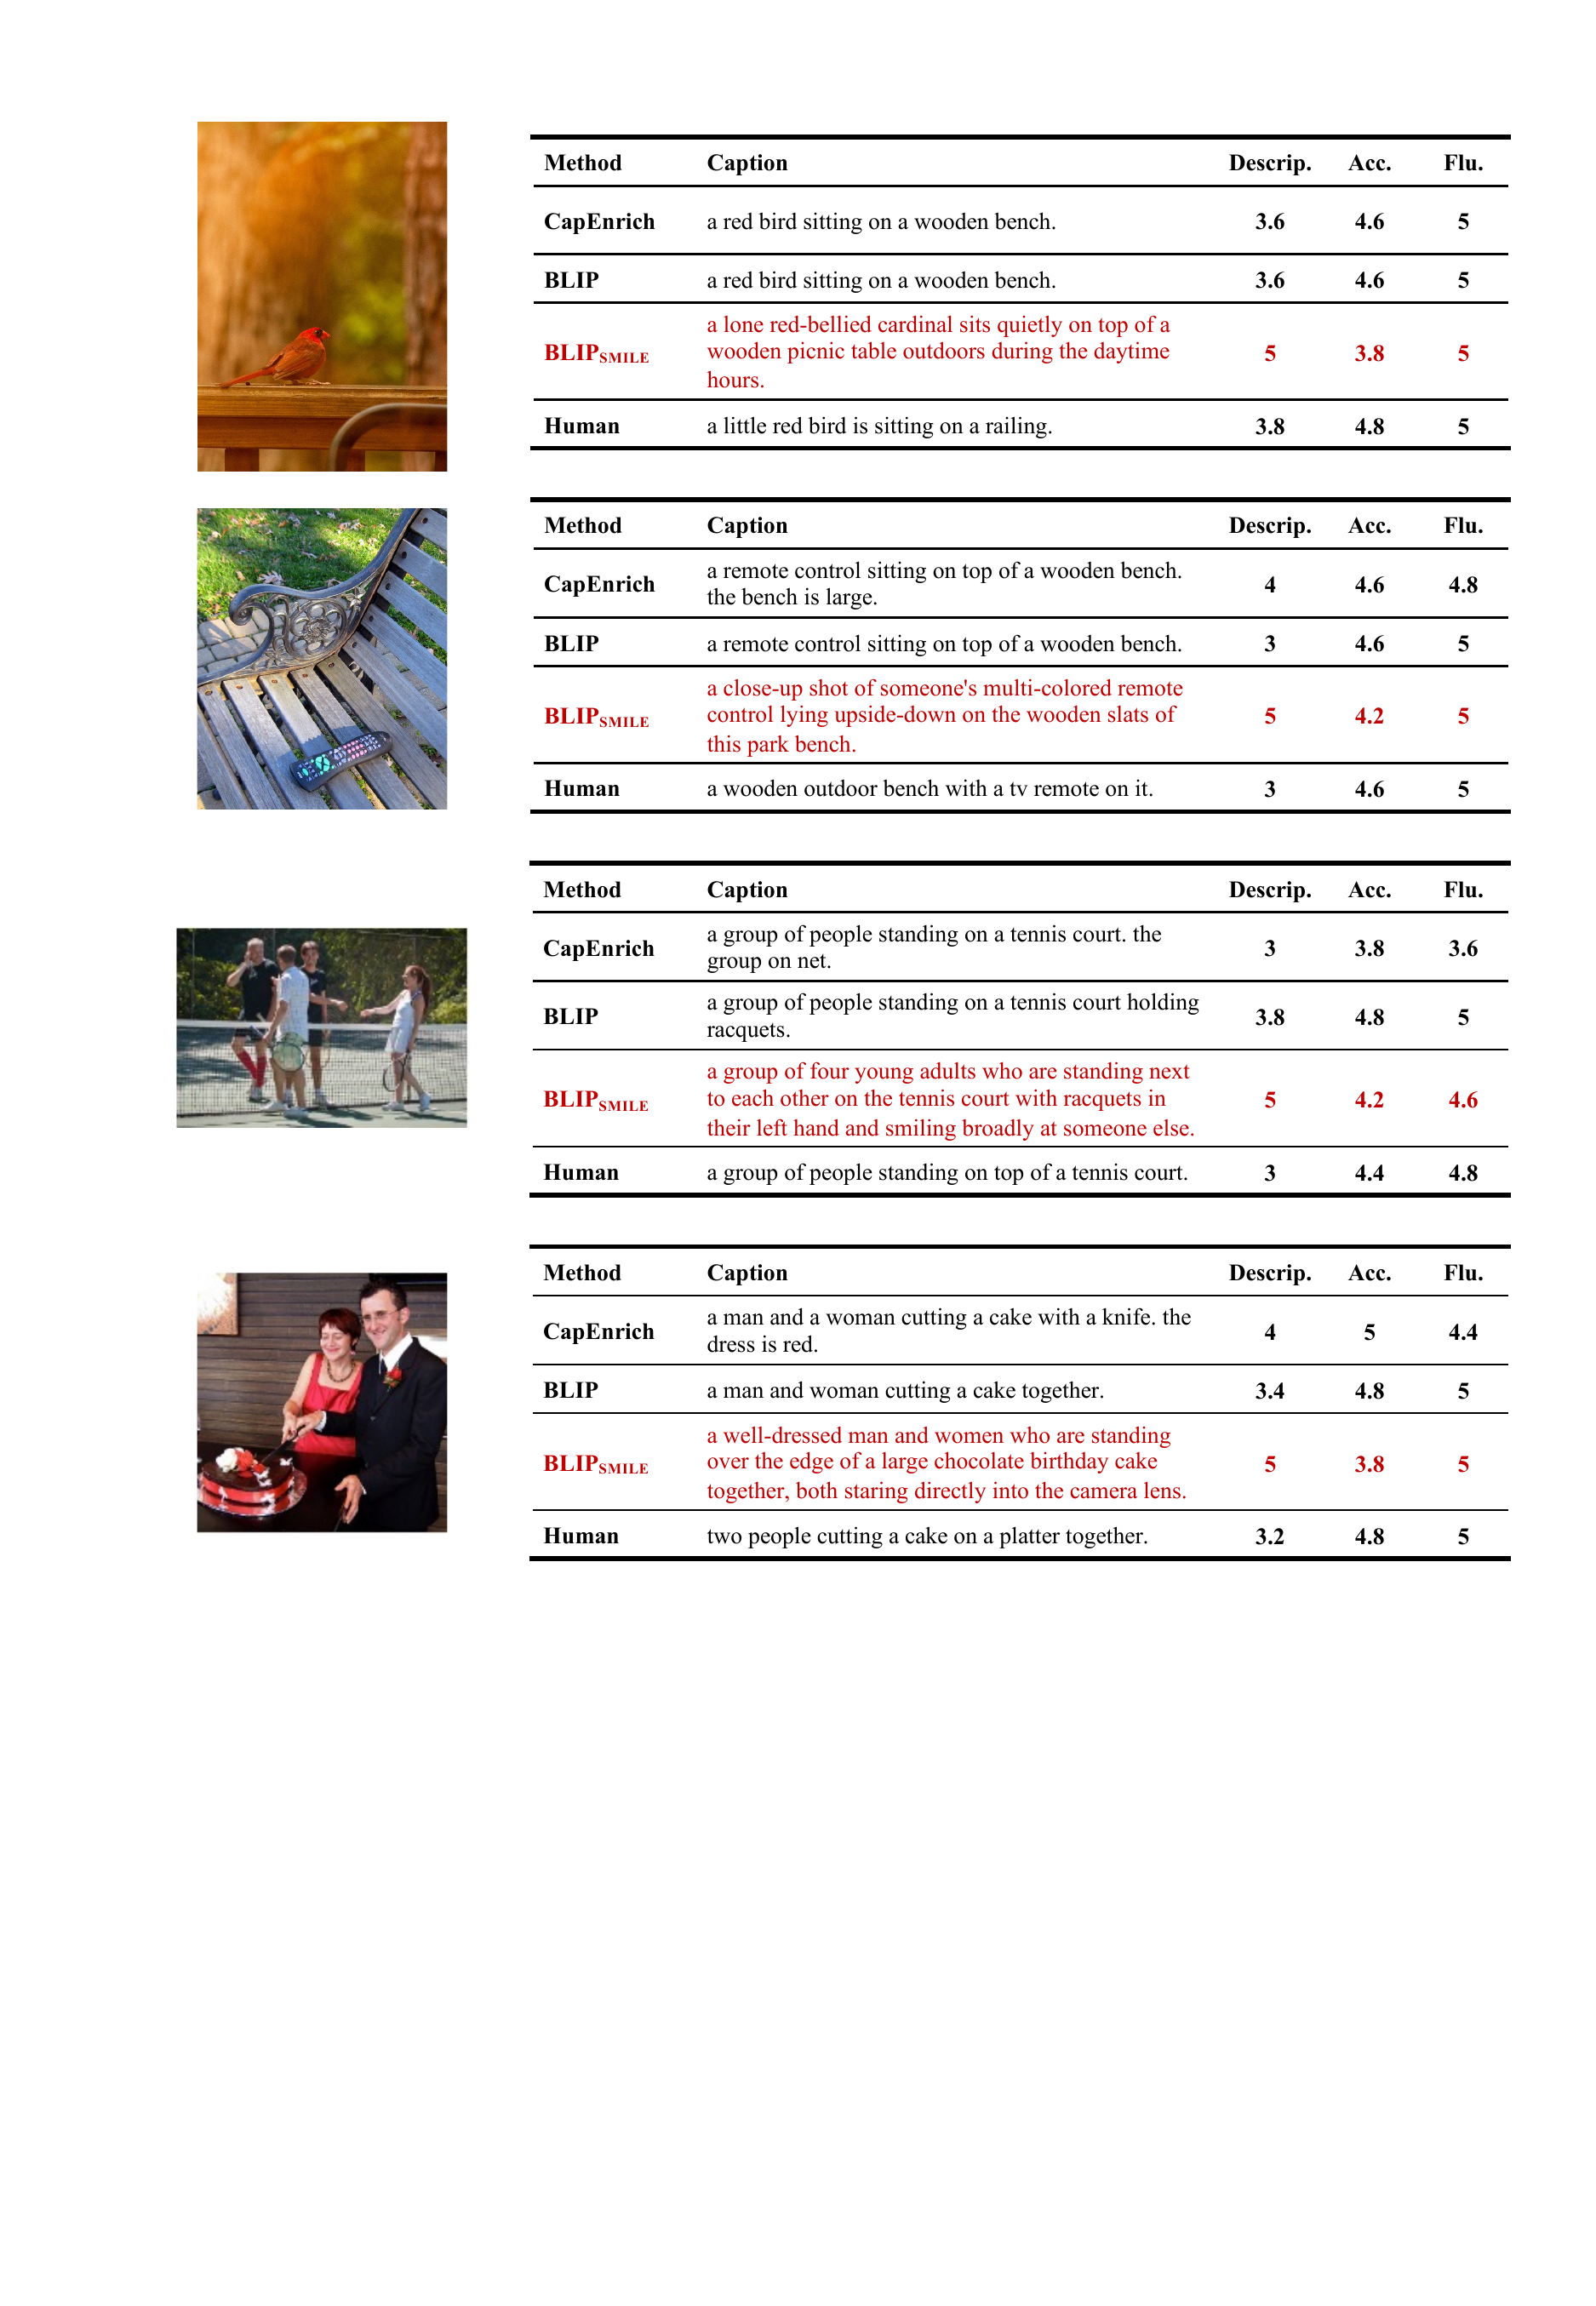}
	\end{center}
	% \vspace{-8pt}
    \caption{Human evaluation cases. The scores are averaged over five annotators. In terms of accuracy, SMILE captions suffer from `talks much errs much', and any minor error can lead to a lower score. In contrast, the other candidates describe much less details, and therefore easily get higher scores.}
	\label{fig:cases}
\end{figure}
